# Supplementary material for: NeRDi: Single-View NeRF Synthesis with Language-Guided Diffusion as General Image Priors
Source: arXiv:2212.03267 source file (2022-12-06)
Supplement: Supplementary file 1 [file a_pumpkin.tex]

\begin{figure}[b]
\centering
\includegraphics[width=.8\linewidth]{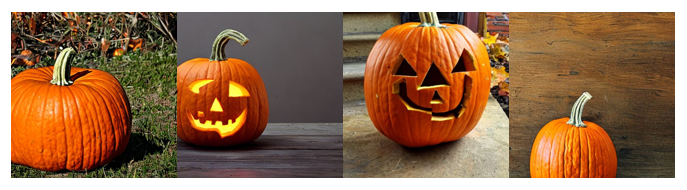}
\caption{Images generated by \cite{Rombach_2022_CVPR} with \texttt{`a pumpkin'}.
}
\label{suppl:fig:a_pumpkin}
\end{figure}
